# Supplementary material for: Tightly-coupled Visual-DVL-Inertial Odometry for Robot-based Ice-water Boundary Exploration
Source: arXiv:2303.17005 source file (2023-08-09)
Supplement: Supplementary file 1 [file 8_appendix.tex]

% !TEX root = main.tex

%%%%%%%%%%%%%%%%%%%%%%%%%%%%%%%%%%%%%%%%%%%%%%%%%%%%%%%%%%%%%%%%%%%%%%%%%%%%%%%%
%%%%%                              Appendix                                %%%%%
%%%%%%%%%%%%%%%%%%%%%%%%%%%%%%%%%%%%%%%%%%%%%%%%%%%%%%%%%%%%%%%%%%%%%%%%%%%%%%%%

\section*{Appendix}
\label{sec:appendix}

aaaa
